# Supplementary material for: Remote determination of the shape of Jupiter's vortices from laboratory experiments
Source: arXiv:2011.11279 ancillary file (2020-11-23)
Supplement: Supplementary file 1 [file Papier_Nat_2019_SI_final.pdf]

# Supplementary Information for

## Remote determination of the shape of Jupiter's vortices from laboratory experiments

**Daphné Lemasquerier[1], Giulio Facchini, Benjamin Favier and Michael Le Bars**

Aix-Marseille Univ, CNRS, Centrale Marseille, Institut de Recherche sur les Phénomènes Hors Équilibre, UMR 7342, 49 rue F. Joliot Curie, 13013 Marseille, France

The Supplementary Information is organized as follows:

**Supplementary Equations**

- In **section 1**, we recall the theoretical framework with more details than in the main manuscript and similarly for the derivation of the theoretical 3D shape of a vortex in our setup;

**Supplementary Methods**

- In **section 2**, we detail the experimental methods. We illustrate them with visualizations and PIV fields (Fig. S1) and velocity profiles (Fig. S2). We provide details about the experimental uncertainties;
- In **section 3**, we detail the numerical methods, the way we initialize our numerical simulations and discuss the stability of the considered vortices;
- In **section 4**, we provide the list of the numerical and experimental non-dimensional parameters (Table S1);

**Supplementary Discussion**

- In **section 5**, we show that the dominant balances at play in numerical simulations are consistent with the hypotheses used to derive the theoretical shape of our vortices;
- In **section 6**, we discuss the long-term evolution of the laboratory vortices. We propose a phenomenological law for the charateristic decay time of the vortex (Eq.[17]);
- In **section 7**, we provide the data and parameters used to apply our laws to Jovian vortices (Tables S2 and S3).
- In **section 8**, we show that if one uses the density anomaly to measure the thickness of the vortex, the latter could be 1.7 times what would be measured using the winds extent, which makes our results consistent with the (unpublished) results of the Juno mission[2].

[1]Corresponding author: lemasquerier.pro@protonmail.com

[2]http://www.nasa.gov/feature/jpl/nasas-juno-probes-the-depths-of-jupiters-great-red-spot

# Supplementary Equations

## 1. Detailed theoretical framework and theoretical laws derivation

### 1.1 Governing equations

Let us first set the theoretical framework in which we stand and define all the parameters and variables that will be used in the following. We consider the flow of an incompressible fluid of constant kinematic viscosity $\nu$ rotating around the vertical axis (oriented upward) at a constant rate $\boldsymbol{\Omega} = \Omega\ \boldsymbol{e}_z$. In cartesian coordinates, we denote the velocity field $\boldsymbol{u} = (u, v, w)_{\boldsymbol{e}_x,\boldsymbol{e}_y,\boldsymbol{e}_z}$. Note that the shear is applied along the $x$ direction, so that consistently with the established plane Couette flow, we designate $x$ and $y$ as the *stream-wise* and *cross-stream* directions respectively. We start from the continuity and Navier-Stokes equations as well as the advection-diffusion equation of the stratifying agent of constant diffusivity $\kappa$ (e.g. salt concentration field in our experiments). The concentration field of this stratifying agent is linearly related to the density field, which hence follows the same advection-diffusion equation. In the Boussinesq approximation and in the rotating frame these read

$$\left.\begin{aligned} &\boldsymbol{\nabla}\cdot\boldsymbol{u} = 0,\\ &\frac{\partial \boldsymbol{u}}{\partial t} + (\boldsymbol{u}\cdot\boldsymbol{\nabla})\boldsymbol{u} + f\boldsymbol{e_z}\times\boldsymbol{u} = -\frac{1}{\rho_0}\boldsymbol{\nabla}p + \frac{\rho}{\rho_0}\boldsymbol{g} + \nu\boldsymbol{\nabla}^2\boldsymbol{u},\\ &\frac{\partial\rho}{\partial t} + (\boldsymbol{u}\cdot\boldsymbol{\nabla})\rho = \kappa\boldsymbol{\nabla}^2\rho, \end{aligned}\right\} \tag{1}$$

where $f = 2\Omega$ is the Coriolis parameter, $\rho$ is the fluid density and $\rho_0$ the mean density of the linear stratification. The stationary solution without any vortex nor plane Couette flow, i.e. the hydrostatic equilibrium of the rotating stratified flow, is

$$\begin{aligned} \bar{\rho}(z) &= \rho_0\left(1 - \tfrac{N^2}{g}z\right),\\ \bar{p}(z) &= p_0 - \rho_0 g z + \tfrac{N^2\rho_0}{2}z^2, \end{aligned} \tag{2}$$

where $N = \sqrt{-g\partial_z\bar{\rho}/\rho_0}$ is the buoyancy frequency corresponding to the initial linear stratification. Defining the density and pressure perturbations as $\delta\rho = \rho(x,y,z,t) - \bar{\rho}(z)$ and $\delta p = p(x,y,z,t) - \bar{p}(z)$ gives the following system of equations for the perturbations in the Boussinesq approximation:

$$\left.\begin{aligned} &\boldsymbol{\nabla}\cdot\boldsymbol{u} = 0,\\ &\frac{\partial \boldsymbol{u}}{\partial t} + (\boldsymbol{u}\cdot\boldsymbol{\nabla})\boldsymbol{u} + f\boldsymbol{e_z}\times\boldsymbol{u} = -\frac{1}{\rho_0}\boldsymbol{\nabla}\delta p - \frac{\delta\rho}{\rho_0}g\boldsymbol{e_z} + \nu\boldsymbol{\nabla}^2\boldsymbol{u},\\ &\frac{\partial\delta\rho}{\partial t} + (\boldsymbol{u}\cdot\boldsymbol{\nabla})\delta\rho = \frac{\rho_0 N^2}{g}w + \kappa\boldsymbol{\nabla}^2\delta\rho. \end{aligned}\right\} \tag{3}$$

Both experimentally and numerically, the shear is added via the action of two rigid boundaries located at $y = (-d, d)$ moving at constant velocity in opposite directions parallel to $x$. Using half the distance between the two shearing boundaries $d$ as the length scale and $1/f$ as the time scale gives the non-dimensional variables $(x, y, z, \boldsymbol{u}', \delta\rho', \delta p')$ such that

$$\begin{aligned} &t = t'/f\\ &(x,y,z) = (x',y',z')d,\\ &(u,v,w) = (u',v',w')df,\\ &\delta\rho = \delta\rho'\rho_0 d f^2/g,\\ &\delta p = \delta p'\rho_0 d^2 f^2. \end{aligned} \tag{4}$$

The corresponding non-dimensional set of equations is

$$\boldsymbol{\nabla}'\cdot\boldsymbol{u'} = 0, \tag{5a}$$

$$\frac{\partial\boldsymbol{u'}}{\partial t'} + (\boldsymbol{u'}\cdot\boldsymbol{\nabla}')\boldsymbol{u'} + \boldsymbol{e}_z\times\boldsymbol{u'} = -\boldsymbol{\nabla}'\delta p' - \delta\rho'\ \boldsymbol{e}_z + \frac{1}{Re}\nabla'^2\boldsymbol{u'}, \tag{5b}$$

$$\frac{\partial\delta\rho'}{\partial t'} + (\boldsymbol{u'}\cdot\boldsymbol{\nabla}')\delta\rho' = N_f^2 w' + \frac{1}{ScRe}\nabla'^2\delta\rho', \tag{5c}$$

where we introduce the Reynolds number $Re = d^2 f/\nu$, the Schmidt number $Sc = \nu/\kappa$ and the ratio of the Brunt-Väisälä frequency to the Coriolis frequency $N_f = N/f$. In the following of the Supplementary Information, we drop the $'$ for the sake of clarity but all the variables are dimensionless.

## 1.2 Theoretical 3D shape of an equilibrium vortex

Following the same method as Aubert et al. (1), we discuss here the theoretical shape of a vortex in our setup. In the inviscid limit, we first derive the unperturbed pressure field corresponding to a rotating plane Couette flow, then we derive the pressure field inside a compact ellipsoidal vortex. We finally invoke pressure continuity between those two fields which leads to an ellipsoid equation for the vortex contour.

We start from the Navier-Stokes equation for the perturbations in the Boussinesq approximation [5b] and neglect the viscous, non-linear and time-dependent terms since we search for a steady, weak, cyclo-geostrophic and hydrostatic equilibrium state. For a linear plane Couette flow $\boldsymbol{U} = (-\sigma y, 0, 0)$, the pressure perturbation is

$$\delta P = \delta P_0 + \frac{\sigma}{2} y^2, \qquad [6]$$

where $\delta P_0$ is a constant. Neglecting diffusivity, viscosity and non-linearities allows to consider discontinuous velocity and density fields. We thus look for a compact ellipsoidal vortex of constant vertical vorticity $\omega_c = 2Ro$, whose velocity field can be written as

$$\boldsymbol{u}_v = Ro \begin{pmatrix} -(1+\beta)y \\ (1-\beta)x \\ 0 \end{pmatrix}, \qquad [7]$$

where $\beta = (a^2 - b^2)/(a^2 + b^2)$ is the equatorial ellipticity of the vortex which goes from 0 for an axisymmetric vortex to 1 for an infinitely stretched ellipse. The stratification inside the vortex is assumed to be linear with a buoyancy frequency $N_c$. The corresponding inviscid pressure field is

$$\begin{aligned} \delta p_v = \delta p_c \quad & + \quad \frac{Ro}{2}(1-\beta)\left[Ro(1+\beta)+1\right] x^2 \\ & + \quad \frac{Ro}{2}(1+\beta)\left[Ro(1-\beta)+1\right] y^2 \\ & - \quad \frac{N_f^2 - N_c^2}{2} z^2, \end{aligned} \qquad [8]$$

where $\delta p_c$ is a constant – the pressure anomaly at the vortex center. While the velocity and the density fields are discontinuous, we require the continuity of the pressure field between the vortex and the surrounding rotating plane Couette flow. Equality between [6] and [8] leads to ellipsoidal surfaces defined by

$$\begin{aligned} & Ro\ (1-\beta)\ [1+(1+\beta)Ro]\ x^2 \\ + \quad & \big(Ro\ (1+\beta)\ [1+(1-\beta)Ro] - \sigma\big)\ y^2 \\ + \quad & \big(N_c^2 - N_f^2\big)\ z^2 = \text{cst}. \end{aligned} \qquad [9]$$

Applying this relation at the points $(x, y, z) = (a, 0, 0)$, $(0, b, 0)$ and $(0, 0, c)$ gives the relations for the ellipticity $\beta$ and the vertical aspect ratio $c/a$ given in the main manuscript:

$$\beta^2 \left(2\frac{Ro_x^2}{\sigma} + 1\right) + 2\beta\left(\frac{Ro_x^2}{\sigma} - 1\right) + 1 = 0, \qquad [10]$$

$$\left(\frac{c}{a}\right)^2 = \frac{Ro_x \left[1 + Ro_x\ \frac{1+\beta}{1-\beta}\right]}{N_c^2 - N_f^2} \qquad [11]$$

where $Ro_x = (1-\beta)Ro$ is the stream-wise Rossby number. In the present study, we focus on anticyclones ($Ro_x < 0$) embedded in an anticyclonic shear ($\sigma < 0$) since it is the situation of the vast majority of Jovian vortices (2).

Note that in terms of scaling analysis, the dimensionless parameters entering those laws are fully consistent with our assumptions. A dissipationless floating vortex is fully characterized by 8 dimensional parameters: its dimensions $a, b$ and $c$, its physical characteristics given by its vorticity $\omega_c$ and the difference between its internal density gradient and the ambient one $N_c^2 - N^2$ and the environment physical characteristics given by the Coriolis frequency $f$, the buoyancy frequency $N$ and the shear $\sigma^*$. According to the $\Pi$-theorem, the whole system is thus characterised by 6 dimensionless numbers, that we chose to be the geometrical parameters given by the equatorial ellipticity $\beta$ and the aspect ratio $c/a$, and the dynamical parameters given

by the Rossby number $Ro = \omega_c/2f$, the dimensionless shear $\sigma = \sigma^*/f$, the dimensionless buoyancy frequency $N_f = N/f$, and the dimensionless buoyancy anomaly $(N_c^2 - N^2)/f^2$. Note that the dimensionless buoyancy frequency does not appear in the scaling laws for the vortex aspect ratio, at least in the Boussinesq approximation considered here. Only the dimensionless buoyancy anomaly does.

The above parameters fully describe the quasi-static, inviscid and diffusion-less problem where our assumptions naturally lead us to neglect other dimensional parameters (the molecular viscosity $\nu$ and the stratifying agent diffusivity $\kappa$). In the full problem (equations 5a-5c), two supplementary non-dimensional parameters are necessary: the Reynolds number $Re = d^2 f/\nu$ and the Schmidt number $Sc = \nu/\kappa$. These parameters $(Re, Sc)$ are not relevant for determining the shape of the vortex, and they will only appear when we discuss the decay of the vortex through time (section 6), which is a completely different question.

# Supplementary Methods

## 2. Detailed experimental methods

### 2.1 Experimental set-up

The experimental set-up used in this study is the same as the one described in Facchini et al. (3), except that we create a vortex within the established linear plane Couette flow. We recall briefly its principal features. A tank ($50 \times 50 \times 70$ cm) is filled with salt water linearly stratified in density using the double bucket method. The tank is mounted on a table that rotates around a vertical axis at a rate $\Omega$. The stratification is measured vertically by sampling the fluid at different heights and measuring the corresponding density with a density-meter. In all the experiments discussed here, we generated stratifications corresponding to a buoyancy frequency $N = 1 \pm 0.1$ rad s$^{-1}$ with a rotation rate $\Omega = 0.5 \pm 0.05$ rad s$^{-1}$ such that $N_f = 1 \pm 0.2$. Note that the topographic $\beta$-effect resulting from the free-surface deformation due to rotation is negligible in our case, the corresponding Rhines scale (1 m) being 10 times larger than the vortices scale (10 cm). To impose a shear in the flow, we use a PVC belt encircling two co-rotating cylinders. Two additional pairs of cylinders allow to stretch out the membrane while keeping a constant gap $2d = 6$ cm between the two shearing sheets.

After placing the shearing device inside the tank, we fill it with stratified salted water. We then gradually increase the rotation rate of the turntable to avoid disturbing the stratification during the spin-up. Note that we measure the stratification before and after each experiment to verify that it was not excessively modified. Once solid body rotation is reached, we activate the shear and wait for the stationary plane Couette profile to establish ($\sim$ tens of minutes).

To create anticyclones in this gap, a one millimeter-diameter capillary tube is linked to a reservoir fixed above the tank. Using gravity fall only, we inject a volume of fluid having a constant density equal to the density at the injection height. In the experiments presented here, we typically inject fluid at mid-height during 6 seconds which corresponds to a volume $V \sim 40$ mL. The parameters of the experimental cases discussed in this study are listed in table S1.

### 2.2 Visualization and particle image velocimetry (PIV)

Velocity field measurements are performed in the equatorial plane of the vortex using particle image velocimetry (PIV). We seed the fluid with 10 $\mu$m-diameter hollow glass spheres and their displacement is followed using a camera fixed in the rotating frame above the tank and looking downward. We use the software DPIVSoft 2010 (4) to extract velocity fields from these measurements. Typically, the field covers an area of $19 \times 7$ cm with a resolution of $210 \times 52$ grid points.

PIV is performed before and during each experiment to measure the imposed shear rate $\sigma$, the vortex streamwise Rossby number $Ro_x$ and the vortex horizontal aspect ratio $a/b$ and ellipticity $\beta$. The shear rate is measured as the slope of the streamwise velocity profiles before the experiment. The streamwise Rossby number is measured as the slope of the cross-stream velocity profiles along $(x, 0, 0)$ at the center of the vortex. For those two quantities $\sigma$ and $Ro_x$, uncertainties are estimated by the least-squares method when fitting the streamwise velocity profiles. At each time step, the vortex horizontal aspect ratio is measured by plotting several streamlines near the vortex center. The variability in the measured aspect ratio of the elliptical streamlines provide us with upper and lower bounds for $a/b$, and hence for $\beta$.

For some experiments we added Rhodamine B, a fluorescent dye, in the injected fluid to follow the vortex evolution in a vertical plane. A second vertical laser plane aligned with the $x$-axis is thus present along with a camera fixed on the side of the tank to record corresponding movies. Note that the two laser sheets could not be switched on simultaneously since this would deteriorate the PIV measurements. For that reason, we do not have a continuous recording of the vertical shape of the vortices but only a few instants per experiment during which we temporarily turned off the horizontal laser plane and switched on the vertical one. To compute the vertical aspect ratio, we binarize the images such that all pixels of intensity above an arbitrary threshold are equal to 1. We fill the holes inside the vortex that are due to PIV particles using the MATLAB *imfill* function. We then use the *regionprops* function to detect all the elliptic patches on the binary image. We extract from it the largest form detected as well as its long and short-axis $a$ and $c$ respectively. To get an uncertainty on these measurements, we apply this procedure to tens of images over a time period during which the vortex shape does not evolve significantly (typically 1-3 seconds). From these measurements we get a mean and a standard deviation which is represented as a vertical error bar on Figure 3b in the main text.

All of the experimental uncertainties are propagated to give the error bars in Figure 3 of the main text. The only parameter for which we have no uncertainty is the vortex stratification $N_c$ which we cannot measure experimentally. The vortex is assumed to have a perfectly mixed interior, that is $N_c = 0$ (see however the discussion in section 5.2 about this assumption).

Fig. S1 shows the typical evolution of a vortex as observed during an experiment in the equatorial plane. We chose a case where Rhodamine B was added to the injection fluid for a better visualization. The corresponding velocity fields deduced from PIV are represented, keeping only one grid point out of three in both directions for clarity. The injected vortex is initially compact, stable and axisymmetric and evolves laminarily towards an elliptic shape under the stretching action of shear. Fig. S2 shows velocity profiles along both $x$ and $y$ for experiments and the reference simulation (see table S1). The

shape evolution is accompanied by a decay of the strength of the vortex, that is a decay of its Rossby number $|Ro|$ visible by the flattening of the slopes of the velocity profiles at $x = 0$ in Figure S2. The longevity of the experimental vortices is of the order of 30 rotations of the turntable, that is $t \sim 30 \times 4\pi \sim 400$ in our dimensionless units.

Additionally, we verify that, similarly to (5), along the $x$ direction (parallel to the shear), the velocity profiles are close to that of a gaussian vortex as defined by equation [12]. This is consistent with (6) who showed that when no net vorticity is introduced by the injection process, gaussian isolated vortices are a good approximation of laboratory vortices. In the $y$ direction the effects of confinement are clearly visible, but the velocity field still resembles some gaussian profile superposed to the background shear. Note that the discontinuous linear model [7] exactly corresponds to the core of our experimental and numerical gaussian vortices.

# 3. Detailed numerical methods

## 3.1 Numerical method

We performed direct numerical simulations (DNS) to compare with our experimental results and extend them to a wider range of parameters. To this aim, we solve the full system of equations [5a-5c] using the open-source spectral element solver Nek5000 (7). These equations are solved in a rectangular box of dimensions $(L_x, L_y, L_z)$=(8,2,4) centered around the origin $(x, y, z) = (0, 0, 0)$ to mimic the experimental setup. The boundary conditions are periodic in both the stream-wise ($x$) and vertical ($z$) directions and rigid no-slip insulating boundaries are imposed in the cross-stream ($y$) direction, i.e. $\boldsymbol{u} = \mp\sigma y \, \boldsymbol{e_x}$ and $\partial_y \delta\rho = 0$ at $y = \pm 1$, where $\sigma$ is the shear rate. The global geometry is partitioned into $\mathcal{E}$ hexahedral elements. Inside each element, velocity, density and pressure perturbations variables are projected onto $\mathcal{N}$-th order Lagrange interpolating polynomials distributed on Gauss-Lobatto-Legendre nodes. For all the results discussed in this paper, the number of elements is $\mathcal{E} \sim 3000$ and we use Lagrange interpolating polynomials of order $\mathcal{N} = 15$ ($\mathcal{N} = 10$ after dealiasing) leading to $\sim 10^7$ grid points. Time integration is performed with a third-order explicit scheme for the advection and buoyancy terms while viscous and dissipative terms are integrated using an implicit third-order scheme.

## 3.2 Initial flow

The simulations are initialized with an established linear plane Couette flow $\boldsymbol{u}(t = 0) = -\sigma y \, \boldsymbol{e}_x + \boldsymbol{u}_v$ where $\boldsymbol{u}_v$ corresponds to an axisymmetric ellipsoidal gaussian vortex centered around the origin, that is

$$\boldsymbol{u}_{v,0}(x, y, z) = Ro_0 \begin{pmatrix} -y \\ x \\ 0 \end{pmatrix} \exp\left( -\left[ \frac{\sqrt{x^2 + y^2}}{a_0} \right]^2 - \left[ \frac{z}{c_0} \right]^2 \right), \qquad [12]$$

where $a_0$ and $c_0$ are respectively the initial horizontal and vertical dimensions of the vortex. For all the results discussed in this paper, we take $a_0 = 0.8$ for the vortex to fit between the two moving boundaries at $y = \pm 1$. The initial vertical extent $c_0$ is the one given by equation [11] with an initial ellipticity $\beta_0 = 0$. The choice of starting with a gaussian vortex is firstly motivated by the experimental results which show that the velocity profiles are nearly gaussian, as discussed in section 2.2. Secondly, we initially ran cases with an initial discontinuous vortex in solid body rotation and with uniform density. We abandoned this method since the very steep initial gradients in the density field would require a too high numerical resolution, namely because of the high Schmidt number of our simulations which would not allow their rapid regularization by diffusion. Finally, $Ro_0 = \omega_{c,0}/2$ is the initial Rossby number of the vortex, $\omega_c$ being the vertical component of the vorticity at the center of the vortex (divided by $f$). We explore the case where the shear and the vortex have the same vorticity sign hence we take $Ro_0 < 0$ and $\sigma < 0$.

Keeping in mind the results of Aubert et al. (1) and Hassanzadeh et al. (8) where the equilibrium shape is determined at zeroth-order by a hydrostatic and cyclo-geostrophic balance, the vortex is simultaneously initialized with an internal stratification of buoyancy frequency $N_{c,0}$. The density perturbation inside of the vortex relatively to the background linear stratification is thus

$$\delta\rho_v(x, y, z, t = 0) = \left[N_f^2 - N_{c,0}^2\right] z \exp\left( -\left[ \frac{\sqrt{x^2 + y^2}}{a_0} \right]^2 - \left[ \frac{z}{c_0} \right]^2 \right). \qquad [13]$$

To be consistent with experiments where the injected fluid is well-mixed, we initialize anticyclones with no internal absolute stratification, that is $N_{c,0} = 0$. Thus, along the rotation axis ($(x, y) = (0, 0)$) and in the vicinity of $z = 0$ the density anomaly is $\delta\rho_{v,0} \sim N_f^2 \, z$.

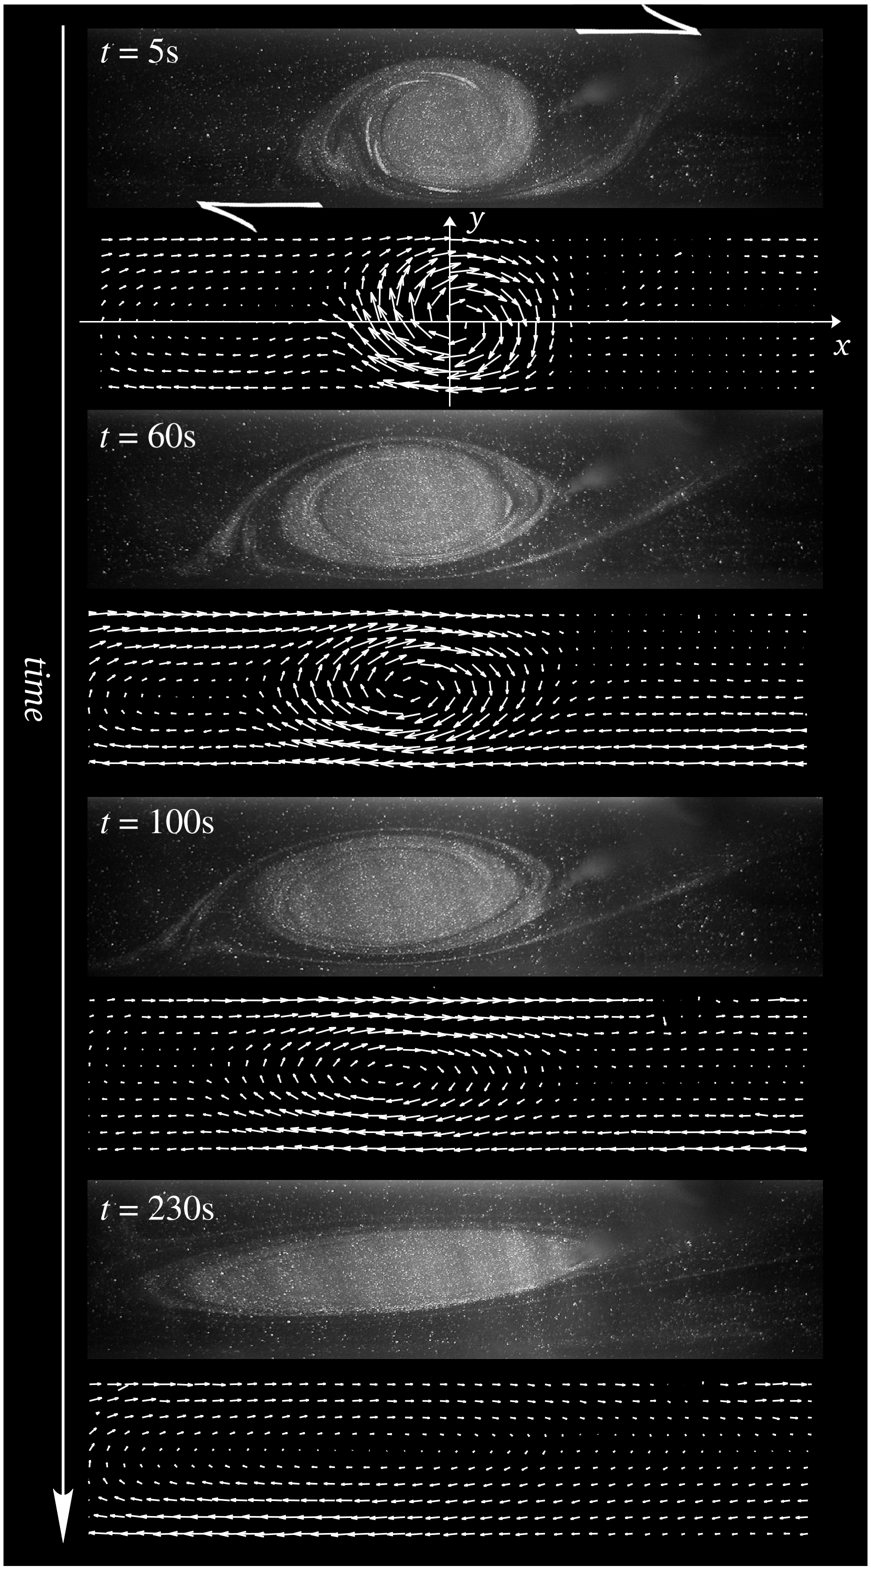


**Figure S1:** Evolution of a sheared anticyclone as observed during our experiments on a horizontal plane. The Rhodamine B added to the injected fluid allows to follow the vortex shape evolution through time. The corresponding PIV vector fields are represented. The shearing boundaries are parallel to the $x$-axis and are located at the borders of the images and vector fields. The injected vortex is initially compact, stable and axisymmetric and evolves laminarily towards an elliptic shape under the action of shear. This shape evolution is accompanied by a decay of the strength of the vortex. Note that at $t = 230$ s, the vortex semi long-axis turns out to be $a \approx 2d$. The shear rate is $\sigma \approx 0.07$ s$^{-1}$. If the vortex was passively advected by the simple shear, it would have reached this extension at a much shorter time $a/\sigma d \approx 2/\sigma \approx 30$ s. On the contrary, if we consider the initial extent $b_0 \approx d/2$, the viscous time scale $d^2/4\nu = 225$ s is of the correct order of magnitude.

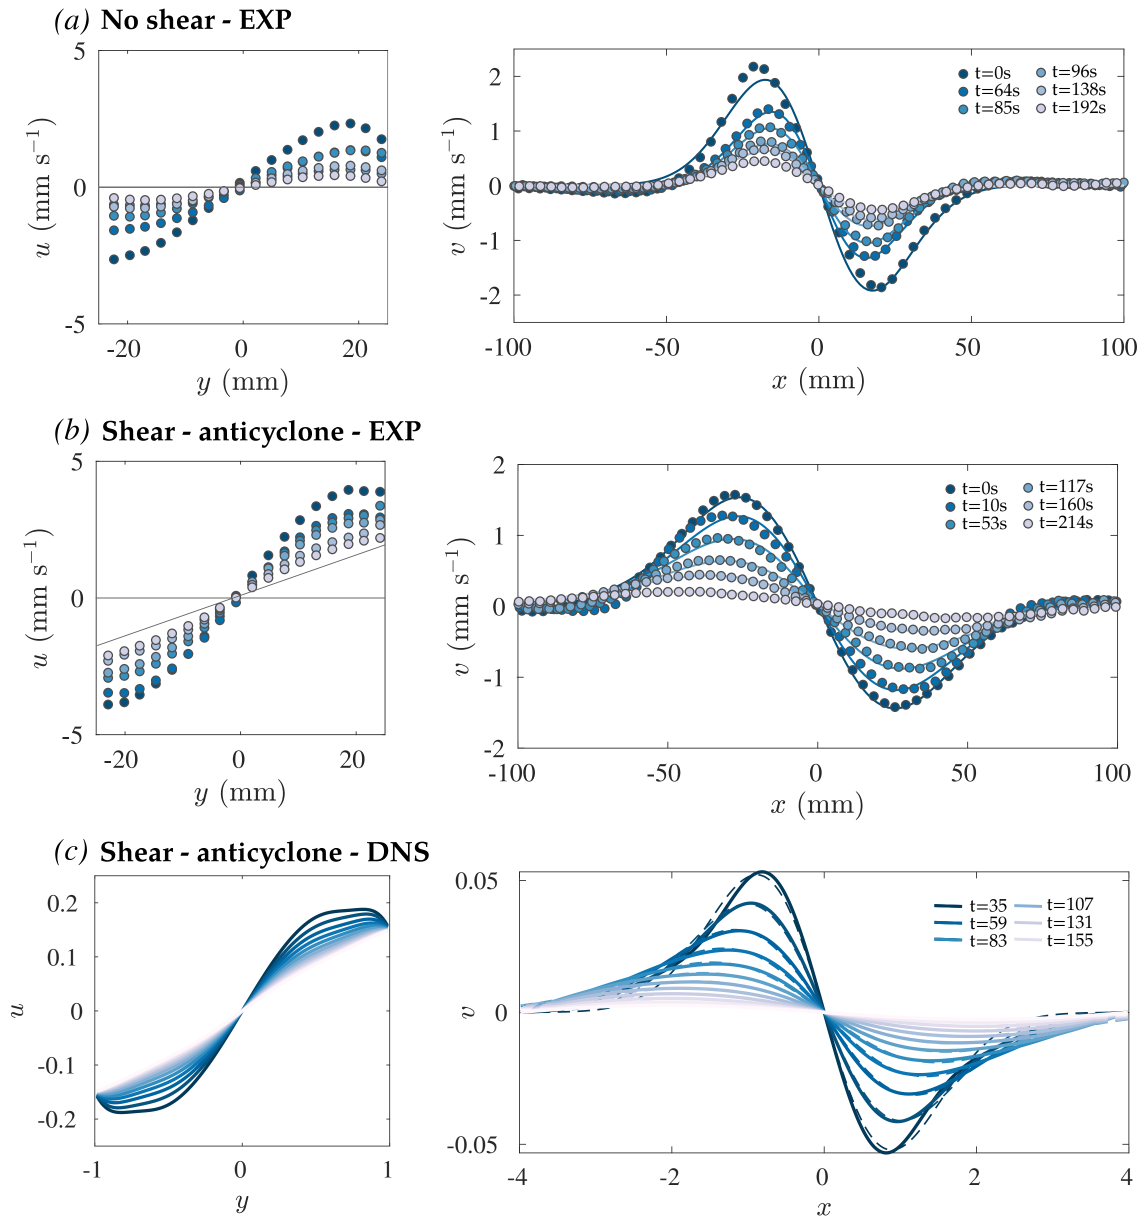


**Figure S2:** *(a,b)* Measured velocity profiles for two anticyclones produced by a 6 seconds injection, *(a)* without shear but with the PVC belt installed so that the vortex is confined in the $y$ direction, and *(b)* with a shear rate $\sigma \approx 0.07$ s$^{-1}$ . The $x$ direction is parallel to the shear direction whereas $y$ is orthogonal to it. The dots are experimental measurements and the lines are the best fitting gaussian profiles. *(c)* Same velocity profiles extracted from the reference simulation (see table S1). The dashed lines are the best-fitting gaussian profiles.

**Table S1:** Experimental and numerical cases parameters. The bold and underlined parameters are those of the reference simulation to which we refer several times in the text. The italic parameters are unstable ones, presumably because of an elliptical instability (see section 3.3).

| | $Re = fd^2/\nu$ | $N_f$ | $Ro_0$ | $\sigma$ | $Sc = \nu/\kappa$ |
|---|---|---|---|---|---|
| Exp | 900 | $\sim 1$ | -0.5 | -0.07 | ~700 |
| Exp | 900 | $\sim 1$ | -0.5 | -0.07 | ~700 |
| Exp | 900 | $\sim 1$ | -0.5 | -0.10 | ~700 |
| Exp | 900 | $\sim 1$ | -0.5 | -0.14 | ~700 |
| Exp | 900 | $\sim 1$ | -0.5 | -0.14 | ~700 |
| Exp | 900 | $\sim 1$ | -0.5 | -0.20 | ~700 |
| Exp | 900 | $\sim 1$ | -0.5 | -0.34 | ~700 |
| DNS | 900 | 1 | -0.45 | -[0.05:0.05:0.45] | 35 |
| DNS | [1800,2700,3600] | 1 | -0.45 | -0.15 | 35 |
| DNS | **900** | **1** | **-0.45** | **-0.15** | [0.07,0.7,7, **35**,70,175] |
| DNS | 900 | 1 | -[0.10:0.05:0.45] | -0.15 | 35 |
| DNS | 900 | [0.50,0.75, *1.33,1.50* *1.75,2.00*] | -0.45 | -0.15 | 35 |

### 3.3 Vortex stability

All the cases reported in the main text and used to verify our model are cases where the vortex is stable. However, we want to mention that we numerically encountered unstable cases even if they are beyond the scope of our study. A wide variety of phenomena can destabilize an axisymmetric pancake-like vortex in a rotating-stratified flow, including gravitational, centrifugal, baroclinic and Gent-Mc Williams instabilities as well as combinations of them (e.g. 9–16). Such instabilities prevented us from exploring cases with strong stratifications, that is $N_f > 1$. Indeed, in those cases the core of the vortex becomes unstable. The study and the origin of this instability are beyond the scope of our study; however, we can locate our unstable cases in the maps of instabilities given in Yim et al. (16). Using their dimensionless parameters definitions, our unstable cases typically have an aspect ratio $\alpha = c_0/a_0 \approx 0.25$, a Froude number $F_h = Ro/N_f \approx 0.23$, a Rossby number $\tilde{Ro} = 2Ro = -0.90$, a Reynolds number of the vortex $\tilde{Re} = RoRe \approx 259$ and a vertical Froude number $F_h/\alpha \approx 0.9$. The low Froude and Rossby numbers are consistent with the Gent-Mc Williams instability described in Yim et al. (16). However our Reynolds number is considerably smaller than the one fixed in their study ($Re$ =10,000) and at such low $Re$, we would rather expect a displacement instability (see figure 5.18 in 17) which is not what we observed. We rather suspect that the observed instability finds its origin in the non-axisymmetric shape of the vortex. Due to the imposed strain field the streamlines in the vortex core are elliptical which may lead to the so-called elliptical instability via a parametric excitation of inertial waves in the core of the vortex (18–20).

## 4. Non-dimensional parameters

Table S1 lists the non-dimensional parameters of all experiments and simulations discussed in this study. The simulations were performed in the ranges $Re \in [900, 3600]$, $Sc \in [0.07, 175]$ and $N_f \in [0.5, 2]$. In the experimental conditions, $Re = 900$, $N_f = 1$ and $Sc \approx 700$. The large experimental value of the Schmidt number is the consequence of the small salt diffusion. To be in the same physical regime without having to impose such a high $Sc$ numerically, we varied it and search for the minimum $Sc$ for which the vortex behavior no longer depends on salt diffusion. As discussed in section 5.2, we show that this is the case as soon as $Sc \geq 35$. All the simulations discussed in this study are thus performed at $Sc = 35$.

# Supplementary Discussion

## 5. Dominant balances

### 5.1 Momentum equations

In this section, we want to show that at order 0, the observations and the dominant physical balances at play at any time during the vortex evolution are consistent with the hypotheses assumed to derive the equilibrium shape.

Firstly, we verify that in the laboratory experiments, after reaching a quasi-static equilibrium state, the formed vortices are indeed ellipsoidal as assumed in section 1.2. To do so, the horizontal aspect ratio of the vortex is computed at each time by plotting several streamlines on the PIV velocity vector fields near the center of the vortex and fitting an ellipse to each of them. It is then verified that there is a factor $(1+\beta)y/(1-\beta)x$ between the magnitude of the velocity along $y$ and $x$ according to equation [7].

Then, we want to verify that the hypothesis of a quasi-cyclogeostrophic and hydrostatic equilibrium is justified. We focus on the results of the reference simulation (table S1) at time $t = 140$. In figure S3$(a,b)$, the projections of equation [5b] onto $\boldsymbol{e}_x$ and $\boldsymbol{e}_y$ along the $(x,0,0)$ and $(0,y,0)$ directions show that the cyclo-geostrophic (or gradient wind) balance

$$\begin{aligned} v\,\partial_y u - v &\approx -\partial_x \delta p, \\ u\,\partial_x v + u &\approx -\partial_y \delta p, \end{aligned} \qquad [14]$$

is indeed verified at zeroth order. Besides, the projection onto $\boldsymbol{e}_z$ (figure S3$c$) is dominated by the hydrostatic balance $\delta\rho \approx -\partial_z \delta p$. We hence verify that the viscous and diffusive effects are negligible to determine the instantaneous shape of the vortex, as well as the vertical velocity $w$. As a consequence, the theoretical pressure field [8] at the core of the vortex fits well those extracted from the numerical simulation, as shown in figure S4. Outside of the vortex, the pressure field recovers the theoretical rotating plane Couette pressure field given by equation [6]. This agreement justifies that we compute the aspect ratios from our simulations using the fact that the pressure perturbation inside the vortex is very close to parabolic in each direction:

$$\left(\frac{a}{b}\right)^2(t) = \frac{(\partial_y^2 \delta p)_c}{(\partial_x^2 \delta p)_c} \quad \text{and} \quad \left(\frac{c}{a}\right)^2(t) = \frac{(\partial_x^2 \delta p)_c}{(\partial_z^2 \delta p)_c}, \qquad [15]$$

where the subscript $c$ means that the derivatives are computed at the center of the vortex.

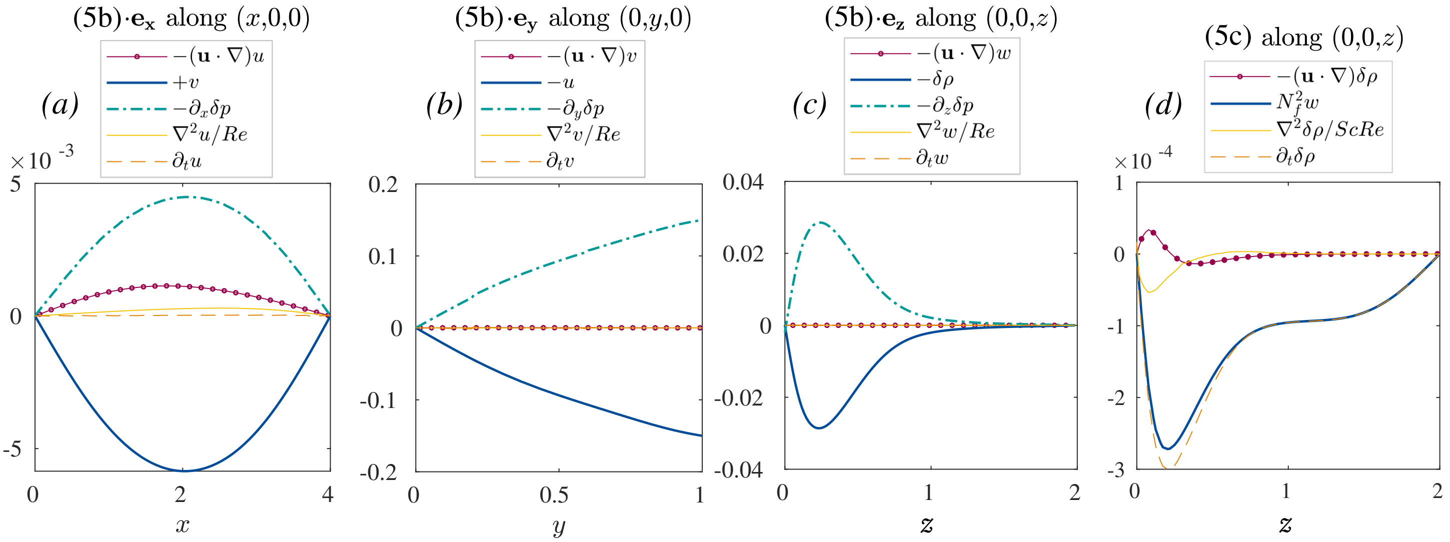


**Figure S3:** Terms of equations [5b] and [5c] for different projections and along different directions. *(a)* First component of [5b] along $x$. *(b)* Second component of [5b] along $y$. These projections show that at zeroth order the system verifies a cyclo-geostrophic equilibrium where the Coriolis and centrifugal forces balances the pressure gradient. *(c)* Third component of [5b] along the $z$ direction showing the predominance of the hydrostatic equilibium $\delta\rho = -\partial_z \delta p$. *(d)* Density anomaly evolution equation [5c] along the $z$ direction.

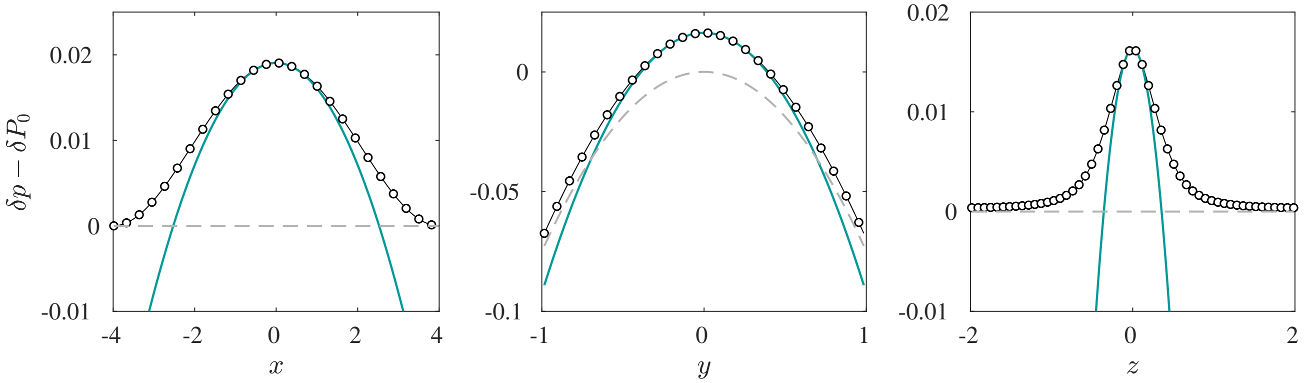


**Figure S4:** Pressure perturbation profiles along ($x$,0,0), (0,$y$,0) and (0,0,$z$). Dots represent results from the reference numerical simulation (parameters given in table S1) at time $t = 140$. The bold green line is the theoretical pressure field [8] inside of the vortex. The dashed grey line is the theoretical plane Couette pressure field [6].

## 5.2 Advection-diffusion of the density anomaly

Figure S3(d) shows the dominant terms in the advection-diffusion equation for the density anomaly. No assumptions were made regarding this equation to derive our theoretical laws. We simply want to mention here that, similarly to Facchini and Le Bars (5), we find that the evolution of the density anomaly of the vortex is due to the vertical advection of the background density field, as demonstrated by the dominant balance $\partial_t \delta\rho \approx N_f^2 w$. This result is important since it can explain the discrepancy between the theory and numerics versus the experimental measurements in Figure 3b of the main text. To compute $(c/a)_{\text{theo}}$, we assume that the vortex is well-mixed i.e. $N_c = 0$. This is true at $t = 0$, and would remain true at larger times if the stratifying agent was diffusing only since diffusion acts on very long timescales given the high Schmidt number of our experiments ($Sc \approx 700$). But we just showed that advection of the background density field dominates over diffusion. This advection is sufficient to lead to significant variations of $N_c$ during the vortex's lifetime, as shown numerically by Figure S5. Even if we work at smaller $Sc$ in our simulations ($Sc = 35$), Figure S5(a-d) shows that no diffusion occurs in the vertical direction, yet the stratification difference vanishes (Figure S5(e)). As a consequence, if we were able to measure $N_c$ experimentally, it would likely increase, leading to a higher value for $(c/a)_{\text{theo}}$ for a given $(c/a)_{\text{mes}}$. It could thus explain the discrepancy in Figure 3b of the main text.

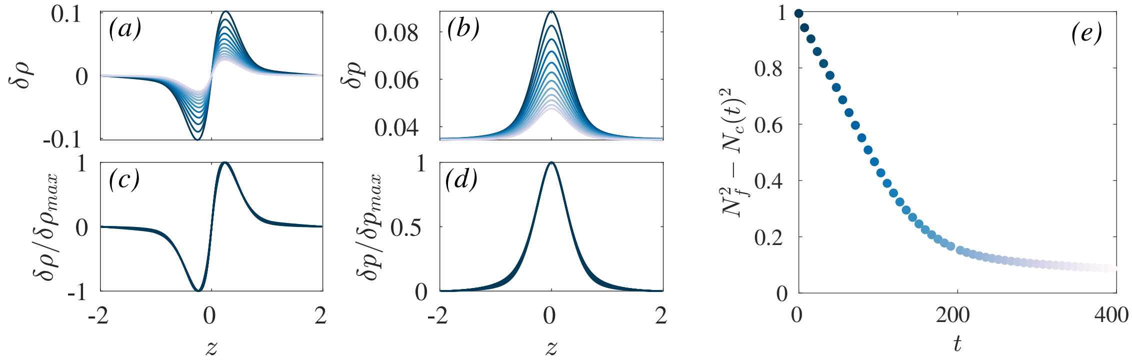


**Figure S5:** *(a,b)* Evolution through time of the density perturbation $\delta\rho$ and the pressure perturbation $\delta p$ along the vertical direction. *(c,d)* The same vertical profiles normalized at each time by their maximum. Once rescaled, all the profiles collapse on the same curve showing that approximately no diffusion occurs in the vertical direction. *(e)* Temporal evolution of the stratification difference between the core of the vortex and the ambient. $N_f^2 - N_c(t)^2$ is computed as the slope of $\delta\rho(0, 0, z, t)$ at $z = 0$.

# 6. Long-term evolution of the vortex

The previous section shows that the time derivatives are negligible compared to the dominant balance. This observation fully supports our hypothesis of a quasi-static equilibrium for the vortex, i.e. a time decoupling between the fast effects that control the equilibrium shape (pressure and azimuthal motion) and the slow dissipative processes that control the time evolution. This assumption is also valid in the Jovian atmosphere where vortices are long-lived. As a result, the equilibrium shape of vortices does not depend on the relevant dissipation mechanism (viscosity in the lab vs. radiative cooling in Jupiter). This is further justified by the work of Hassanzadeh et al. (8) which showed numerically that the laws for the vortex shape in the absence of shear are valid regardless of the dominant dissipation process.

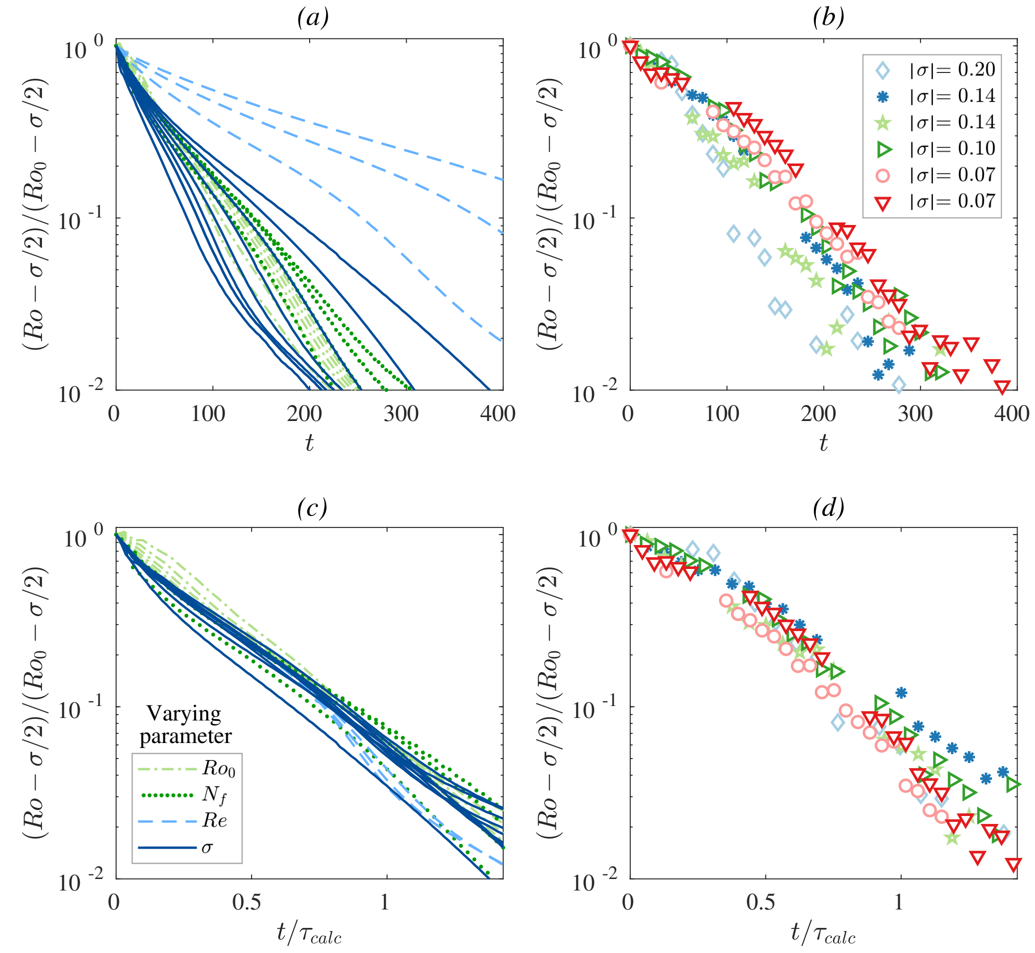


**Figure S6:** Vorticity decay inside the vortex as a function of *(a,b)* the non-dimensional time and *(c,d)* the time normalized by the theoretical decay time given by equation [17]. *(a,c)* Numerical simulations with different shear rates (dark blue, —), $Re$ (light blue, - - -), $Ro_0$ (light green, $- \cdot -$) and $N_f$ (dark green, $\cdots$) compared to the reference case (see table S1). *(b,d)* Experiments with different shear rates.

Even if it is not relevant for determining the shape of the vortex, we address here the question of the vortex decay for completeness of our experimental and numerical study. Note however that contrary to the quasi-static equilibrium shape, the following results only apply to our laboratory and numerical vortices, not to Jovian ones. Indeed, the Reynolds number of our laboratory vortices is too small, the background flow is not turbulent, and the density dissipation is related to salt diffusion, not thermal radiation.

As previously mentioned, the shape evolution is accompanied by a decay of the strength of the vortex, that is a decay of its Rossby number $|Ro|$ visible by the flattening of the slopes of the velocity profiles at $x = 0$ in Figure S2. The first row of Figure S6 represents the decay of the normalized Rossby number of the vortex as a function of time for different numerical simulations and experiments. The longevity of the experimental vortices is of the order of 30 rotations of the turntable, that is $t \sim 30 \times 4\pi \sim 400$ in our dimensionless units.

In the absence of shear and confinement, Facchini and Le Bars (5) showed that in the limit where the Schmidt number $Sc \gg 1$, the Ekman number $Ek = \nu/(2\Omega L^2) \ll 1$, the Rossby number $Ro \ll 1$ and $N_f = 1$, the pressure field verifies a radial diffusion equation. As long as the density diffusion does not play an important role, the dynamical evolution of the vortex is thus expected to occur mainly in horizontal directions. This result is fundamental since it is one of the keys to understand the longevity of such systems: even for a very flat vortex, the relevant distance $L$ to estimate its longevity ($T = L^2/\nu$) is the horizontal extent of the vortex (i.e. the largest) rather than the vertical one (i.e. the shortest). In figure S5*(a-d)*, we verify with our reference DNS that this result still holds in our configuration. We plot successive profiles of the density and pressure perturbations along the centered vertical direction $(0, 0, z)$. These plots show their decay through time with no diffusion in the vertical direction since all the profiles collapse when normalizing them at each time with their maximum.

However, in our case, when no shear is present, confinement prevents spreading in the cross-stream direction as seen in Figure S2. The decaying law $Ro(t)$ should thus be different. We indeed verified that $\sqrt{Ro_0/Ro - 1}$ is not linear in time contrary to what is expected for a radial diffusion of pressure. Similarly to Facchini and Le Bars (5), we find that the evolution of the density anomaly of the vortex is due to the vertical advection of the background density field, as demonstrated by the dominant balance $\partial_t \delta\rho \approx N_f^2 w$ shown in Figure S3*(d)*. However, the balances in the momentum equation significantly differ

at order 1 (order 0 being the cyclo-geostrophic equilibrium): we verified that the diffusive term is not mainly balanced by the Coriolis term. Physically, this means that in our case viscosity does not mainly generate a radial secondary circulation but rather directly acts on the vortex temporal evolution through the viscous coupling with the shearing boundaries. This result further justifies that besides the pure effect of confinement, the physical process at play governing the vortex evolution differs from the case where no shear is applied. We hence expect the decay time to vary significantly with the shear rate.

We performed a numerical systematic study to understand how the decay time varies with key parameters. For each simulation and experiment, we measure a characteristic decay time $\tau_{\text{mes}}$ corresponding to the time for which the vortex has lost 95% of its initial vorticity, that is $(Ro(\tau_{\text{mes}}) - \sigma/2)/(Ro_0 - \sigma/2) = 0.05$. The results are represented in Figure S7 along with their best fits. First, the decay time is proportional to the Reynolds number $Re$, which confirms that the main dissipation mechanism at play is a viscous one. One also notices that the decay rate is independent on the Schmidt number (hence on salt diffusion) once $Sc \geq 35$.

Then, since the dominant balance for the evolution of the density anomaly associated with the vortex is $\partial_t \delta\rho \approx N_f^2 w$, one would expect the characteristic time to be of the form $\tau \sim \delta\rho/(N_f^2\ W)$ where $W$ is the characteristic vertical velocity. Then, since the vortex is well-mixed at the beginning of an experiment, the density anomaly scales as $\delta\rho \sim N_f^2 c_0$ (see section 3.2), hence $\tau \sim c_0/W$: it is quite intuitive that for a given vertical advection of the background density field, it takes more time to destroy the density anomaly of the vortex if it extends more vertically. Now, considering $a_0 \sim 1$ and equation [11], $c_0 \sim (-Ro_0(1 + Ro_0))^{1/2}/N_f$, which leads to

$$\tau \sim \frac{(-Ro_0(1 + Ro_0))^{1/2}}{N_f\ W}. \qquad [16]$$

We verified numerically this scaling by varying the initial Rossby number of the vortex while keeping the other parameters constant. Figure S7*a* shows indeed that the measured decay time $\tau_{\text{mes}}$ is proportional to $(-Ro_0(1 + Ro_0))^{1/2}$.

Then, relation [16] suggests a dependence of the decay time on the background stratification. In the absence of shear, Facchini and Le Bars (5) showed that the decaying solution of their full linear model is bounded by two self-similar solutions corresponding to a radial diffusion of pressure of characteristic times $\tau_1 = 2/Ek$ and $\tau_2 = 2/(Ek\ N_f^2)$. When the background stratification is stronger, the vortex decays faster, and conversely for a weaker stratification. However, we do not observe here any quantitative tendency of how the decay rate varies with $N_f$. Numerically, we ran several simulations with $N_f$ ranging from 0.5 to 2. As explained in section 3.3, the cases with $N_f > 1$ were unstable. For $N_f < 1$, no instability occurs and the changes in the vortex decay rate are too small to be significant or to deliver a clear tendency. From the previous estimate [16], it is not surprising that a clear scaling is not obtainable. Indeed, we expect the vertical velocity $W$ to decrease as the stratification is stronger (higher $N_f$), and increase as it is weaker (lower $N_f$). Consequently, when increasing (or decreasing) $N_f$, there can be a compensation ($N_f W \sim \text{cst}$) leading to a non-significant variation of the decay time.

Finally, we explored the influence of the shear rate $\sigma$. Both the experiments and the DNS show that $\tau_{\text{mes}} \propto \sigma^{-1/2}$ (figure S7*a*). Besides, this scaling still holds when we remove both rotation and stratification of the background flow (i.e. when we simulate sheared columnar vortices). The scaling law of the decay rate with shear is thus independent of the two other physical ingredients of our study and solely depends on how the vortex reconnects with the no-slip shearing boundaries.

In figure S7*b*, the measured decay time is plotted against the phenomenological one. A rather convincing linear 1:1 relationship is found when a prefactor of $\sim 0.14$ is added to the calculated $\tau$, thus giving the final phenomenological relation

$$\tau_{\text{calc}} \approx 0.14\ Re\ \left(\frac{Ro_0(1 + Ro_0)}{\sigma}\right)^{1/2}. \qquad [17]$$

In figure S6, we show that the Rossby decay curves indeed collapse when rescaling the time by $\tau_{\text{calc}}$ for both the simulations and the experiments.

Note again that this scaling law for the time evolution is relevant for our laboratory vortices only, which have a Reynolds number much smaller that Jovian ones. Nevertheless, the zeroth order equilibrium describing the shape of vortices does not depend on their time evolution: it is equally valid for laboratory and Jovian vortices, as shown in the main text.

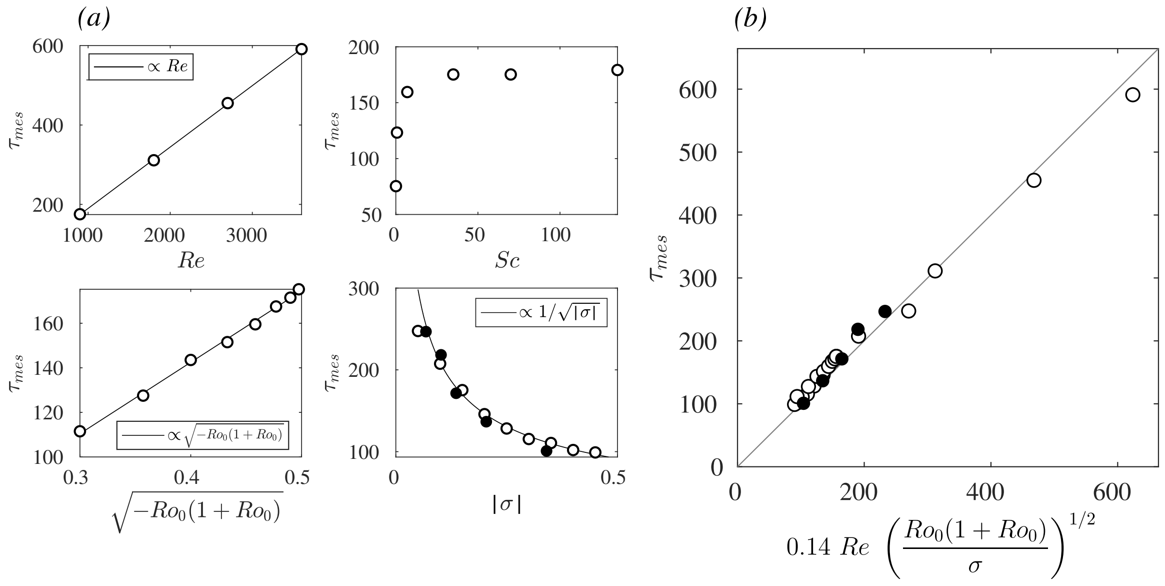


**Figure S7:** *(a)* Evolution of the characteristic decay time as a function of the Reynolds number $Re$, the Schmidt number $Sc$, $(-Ro_0(1+Ro_0))^{1/2}$ and the absolute value of the shear rate $|\sigma|$. The decay time is defined as the time for which the vortex has lost 95% of its initial vorticity, that is $(Ro(\tau)-\sigma/2)/(Ro_0-\sigma/2)=0.05$. *(b)* Measured decay time as a function of the theoretical decay time inferred from the systematic. Numerical simulations are represented by open circles while the black dots represent five experiments with different shear rates $\sigma$.

# 7. Data and estimates for application to Jovian vortices

In this section, we report the data and parameters used to apply our model to four Jovian anticyclones. The Great Red Spot (GRS) has been observed in Jupiter's southern hemisphere for hundreds of years (21). In table S2, we report data for the GRS measured during the *Voyager 1* mission in 1979 (22–24). Contrary to the GRS, Jupiter's Oval BA was created recently after the merger of three White Ovals between 1998 and 2000. We report in table S2 data about the Oval BA measured during the *New Horizons* mission in 2007 (25), as well as data from *Galileo* about two of the three vortices that merged, the Ovals DE and BC, in 1997 (25–27).

To apply our model to Jovian vortices, four parameters are required: the longitudinal Rossby number of the vortex $Ro_x$, the shear rate $\sigma$, the Coriolis frequency $f$ and the stratification difference between the vortex and the surrounding atmosphere $N_c^2 - N^2$. The methods employed to estimate each parameter are available in the Methods section of the main text. Here, we report in Table S2 all the deduced parameters, as well as the predictions of our model:

- the predicted horizontal ellipticity ($\beta_{\text{calc}}$) or aspect ratio ($(a/b)_{\text{calc}}$) of the vortex deduced from equation [10];
- the predicted half-thickness $c_{\text{calc}}$ of the vortex deduced from equation [11]. Note that $c_{\text{calc}}$ is computed using the *estimated* value of $\beta$ in equation [11], whereas for $c'_{\text{calc}}$ we use the *measured* value of $\beta$.

In Table S3, we report the parameters and references used to compute the GRS aspect ratios as a function of time since 1979 (Fig.5 of the main text).

**Table S2:** Estimation of the horizontal and vertical aspect ratios of the Great Red Spot (GRS) in 1979, the Oval BA in 2007 and the Oval DE and BC in 1997. The horizontal aspect ratios ($a/b$) are computed using equation [10] and the vertical ones ($c/a$) using equation [11].

| Refs. | **GRS** *Voyager 1 (1979)* (22–24) | **Oval BA** *New Horizons (2007)* (25) | **Oval DE** *Galileo (1997)* (25) | **Oval BC** *Galileo (1997)* (26, 27) |
|---|---|---|---|---|
| *Rotation, stratification* | | | | |
| $f \cdot 10^4$ (rad/s) | 1.35 | 1.92 | 1.92 | 1.92 |
| $N^2 - N_c^2 \cdot 10^5$ (rad$^2$/s$^2$) | 2.53 ± 1.16 | 1.78 ± 1.19 | 1.78 ± 1.19 | 1.78 ± 1.19 |
| *Vortex dimensions* | | | | |
| $a$ (km) | 9000 | 3350 | 2950 | 4890 |
| $b$ (km) | 4667 | 2750 | 2200 | 2930 |
| $(a/b)_{\text{mes}}$ | **1.93** | **1.22** | **1.34** | **1.67** |
| $\beta_{\text{mes}}$ | 0.58 | 0.20 | 0.29 | 0.47 |
| *Vortex velocities* | | | | |
| $Ro_x \cdot 10^2$ [a] | -15.41 ± 0.58 | -18.78 ± 1.11 | -19.13 ± 1.23 | -12.78 ± 2.13 |
| *Shear* | | | | |
| $\sigma \cdot 10^5$ (s$^{-1}$) | 1.50±0.16[b] | 1.54±0.07[c] | 1.57±0.23[d] | 1.57±0.23[d] |
| $\sigma/f \cdot 10^2$ | -11.11±1.17 | -8.02±0.36 | -8.18±1.20 | -8.18±1.20 |
| *Computed dimensions* | | | | |
| $\beta_{\text{calc}}$ | 0.55 ± 0.05 | 0.35 ± 0.05 | 0.35 ± 0.08 | 0.47 ± 0.15 |
| $(a/b)_{\text{calc}}$ | **1.84** ± 0.14 | **1.45** ± 0.08 | **1.44** ± 0.14 | **1.67** ± 0.30 |
| $(c/a)_{\text{calc}} \cdot 10^3$ | $8.84^{+3.58}_{-1.73}$ | $15.37^{+12.08}_{-3.82}$ | $15.45^{+12.50}_{-4.00}$ | $13.04^{+11.58}_{-3.88}$ |
| $c_{\text{calc}}$ (km) | $80^{+32}_{-16}$ | $51^{+40}_{-13}$ | $46^{+45}_{-12}$ | $64^{+56}_{-19}$ |
| $(c/a)'_{\text{calc}} \cdot 10^3$ | $8.66^{+3.30}_{-1.58}$ | $16.75^{+12.85}_{-4.03}$ | $16.12^{+12.27}_{-3.85}$ | $13.06^{+10.28}_{-3.41}$ |
| $c'_{\text{calc}}$ (km) | $78^{+30}_{-14}$ | $56^{+43}_{-14}$ | $48^{+36}_{-11}$ | $64^{+50}_{-17}$ |

[a] longitudinal Rossby number. When meridional velocity profiles inside the vortices are available (Oval BA and Oval DE), it is determined by a linear fit in the vortex core. Otherwise, we divide the peak North-South velocities by the vortex semi-major axis $a$ (Oval BC) or the vortex collar width (GRS, see Table S3). The velocity profiles used are taken from (25) for the Oval BA and DE, and the peak velocities from (26) for the GRS and (27) for the Oval BC.
[b] estimated by a linear fit on the wind profile at the GRS latitude, given in (22).
[c] estimated from zonal winds data in 2009 provided in Tollefson et al. (30).
[d] estimated from zonal winds data obtained from Voyager 1 and 2 images (29).

**Table S3:** Parameters and references used to compute the GRS aspect ratios as a function of time since 1979 (Figure 5 of the main text). The Coriolis parameter $f$, the stratification difference $N^2 - N_c^2$ and the shear rate $\sigma$ are not indicated because they are taken equal to the values given in Table S2.

| | **1979** | **1996** | **2000** | **2006** | **2012** | **2015** | **2016** | **2017** |
|---|---|---|---|---|---|---|---|---|
| | *Voyager 1* | *Galileo* | *Galileo* | *HST* | *HST* | *HST* | *HST* | *HST* |
| Refs. | (26) | (23) | (23) | (28) | (24) | (24) | (24) | (24) |
| $a$ (km) | $9200 \pm 400$ | $8927 \pm 400$ | $8377 \pm 400$ | $8376 \pm 400$ | $4527 \pm 400$ | $4939 \pm 400$ | $4650 \pm 400$ | $4321 \pm 400$ |
| $a_c$ (km) | $5195 \pm 400$ | $4233 \pm 400$ | $4417 \pm 400$ | $4051 \pm 400$ | $3292 \pm 400$ | $3704 \pm 400$ | $3704 \pm 400$ | $3704 \pm 400$ |
| $a/a_c$ | $1.77 \pm 0.21$ | $2.11 \pm 0.29$ | $1.90 \pm 0.26$ | $2.07 \pm 0.30$ | $1.38 \pm 0.29$ | $1.33 \pm 0.25$ | $1.26 \pm 0.24$ | $1.17 \pm 0.23$ |
| ${Ro_x}^a \cdot 10^2$ | $15.41 \pm 2.59$ | $21.54 \pm 3.75$ | $22.08 \pm 3.79$ | $23.09 \pm 4.00$ | $22.11 \pm 4.90$ | $19.65 \pm 4.09$ | $20.63 \pm 4.19$ | $19.65 \pm 4.09$ |

[a] For the GRS in 1996, 2000 and 2006, the longitudinal Rossby number is computed by a linear fit on the meridional velocity profiles (23, 28) inside the anticyclonic collar. For the other dates, we use $Ro_x \approx \frac{V_{max}}{a_c f}$ where $V_{max}$ is the mean peak meridional velocity along an East-West profile and $f = 1.374$ rad s$^{-1}$.

## 8. Roots of the vortex

We conclude this Supplementary Information by an illustration of the potential difference between the dynamical thickness of the vortex and the thickness of the density anomaly associated with it. We expect the extent of the density anomaly to be larger than the extent of the wind because, starting from the vortex midplane at $z = 0$, the winds decay when going deeper within the vortex. On the contrary, the density anomaly increases from the center of the vortex down to its bottom because the vortex is under-stratified relative to the ambient, with no anomaly at the center. At the bottom of the vortex, there is no more winds (by definition), but at that location the density anomaly is the highest, and will just begin to reconnect with the ambient stratification.

To make it more quantitative, one can start with equations [12] and [13] in the case of an axisymmetric gaussian vortex:

$$u_\theta(r,z) = Ro\ r\ \exp\left(-\left[\frac{r}{a_0}\right]^2 - \left[\frac{z}{c_0}\right]^2\right), \quad [18]$$

$$\delta\rho(r,z) = (N_f^2 - N_c^2)\ z\ \exp\left(-\left[\frac{r}{a_0}\right]^2 - \left[\frac{z}{c_0}\right]^2\right). \quad [19]$$

At any radius, the ratio of the velocity and density anomalies relative to their maximum are

$$\frac{u_\theta}{u_{\theta,max}} = \exp\left(-\left[\frac{z}{c_0}\right]^2\right), \quad [20]$$

$$\frac{\delta\rho}{\delta\rho_{max}} = \sqrt{2}\frac{z}{c_0}\exp\left(-\left[\frac{z}{c_0}\right]^2 + \frac{1}{2}\right). \quad [21]$$

The density anomaly only starts to decay at $z = c_0/\sqrt{2}$ whereas the velocities decrease from $z = 0$. In both cases, the inflection point in the decreasing part of the profiles corresponds to a decrease of $\sim 40\%$ from the maximum value. But for the velocities the inflection point is located at $z = \frac{c_0}{\sqrt{2}}$ whereas it is reached at $z = \sqrt{\frac{3}{2}}c_0$ for the density anomaly, that is at a distance $\sqrt{3} \sim 1.7$ times larger.

Fig. S8 represents the cross-stream velocity $v$ and the density anomaly $\delta\rho$ on several horizontal slices along $z$ for the reference numerical simulation. The density anomaly clearly spreads more vertically than the cross-stream velocity, even if we stand in a regime where it diffuses less (i.e. $Sc \gg 1$). For instance, a decay of 95% relatively to the max value is reached at $|z| \approx 0.9$ in terms of density and at $|z| \approx 0.5$ in terms of velocity. This justifies that our results (GRS thickness of $\sim 148$ km) are not incompatible with the latest (unpublished) Juno imaging[3] which seems to indicate a 300-km thickness for the GRS roots, as discussed in the main text.

## References


[1] Aubert, O., Le Bars, M., Le Gal, P. & Marcus, P. S. The universal aspect ratio of vortices in rotating stratified flows: Experiments and observations. *Journal of Fluid Mechanics* **706**, 34–45 (2012).

[2] Vasavada, A. R. & Showman, A. P. Jovian atmospheric dynamics: An update after *Galileo* and *Cassini*. *Reports on Progress in Physics* **68**, 1935–1996 (2005).

[3] Facchini, G., Favier, B., Le Gal, P., Wang, M. & Le Bars, M. The linear instability of the stratified plane Couette flow. *Journal of Fluid Mechanics* **853**, 205–234 (2018).

[4] Meunier, P. & Leweke, T. Analysis and treatment of errors due to high velocity gradients in particle image velocimetry. *Experiments in fluids* **35**, 408–421 (2003).

[5] Facchini, G. & Le Bars, M. On the lifetime of a pancake anticyclone in a rotating stratified flow. *Journal of Fluid Mechanics* **804**, 688–711 (2016).

[6] Kloosterziel, R. C. On the large-time asymptotics of the diffusion equation on infinite domains. *Journal of Engineering Mathematics* **24**, 213–236 (1990).

[7] Fischer, P. F., Lottes, J. W. & Kerkemeier, S. G. Nek5000 Web page. http://nek5000.mcs.anl.gov (2008).

[8] Hassanzadeh, P., Marcus, P. S. & Le Gal, P. The universal aspect ratio of vortices in rotating stratified flows: Theory and simulation. *Journal of Fluid Mechanics* **706**, 46–57 (2012).


[3] http://www.nasa.gov/feature/jpl/nasas-juno-probes-the-depths-of-jupiters-great-red-spot

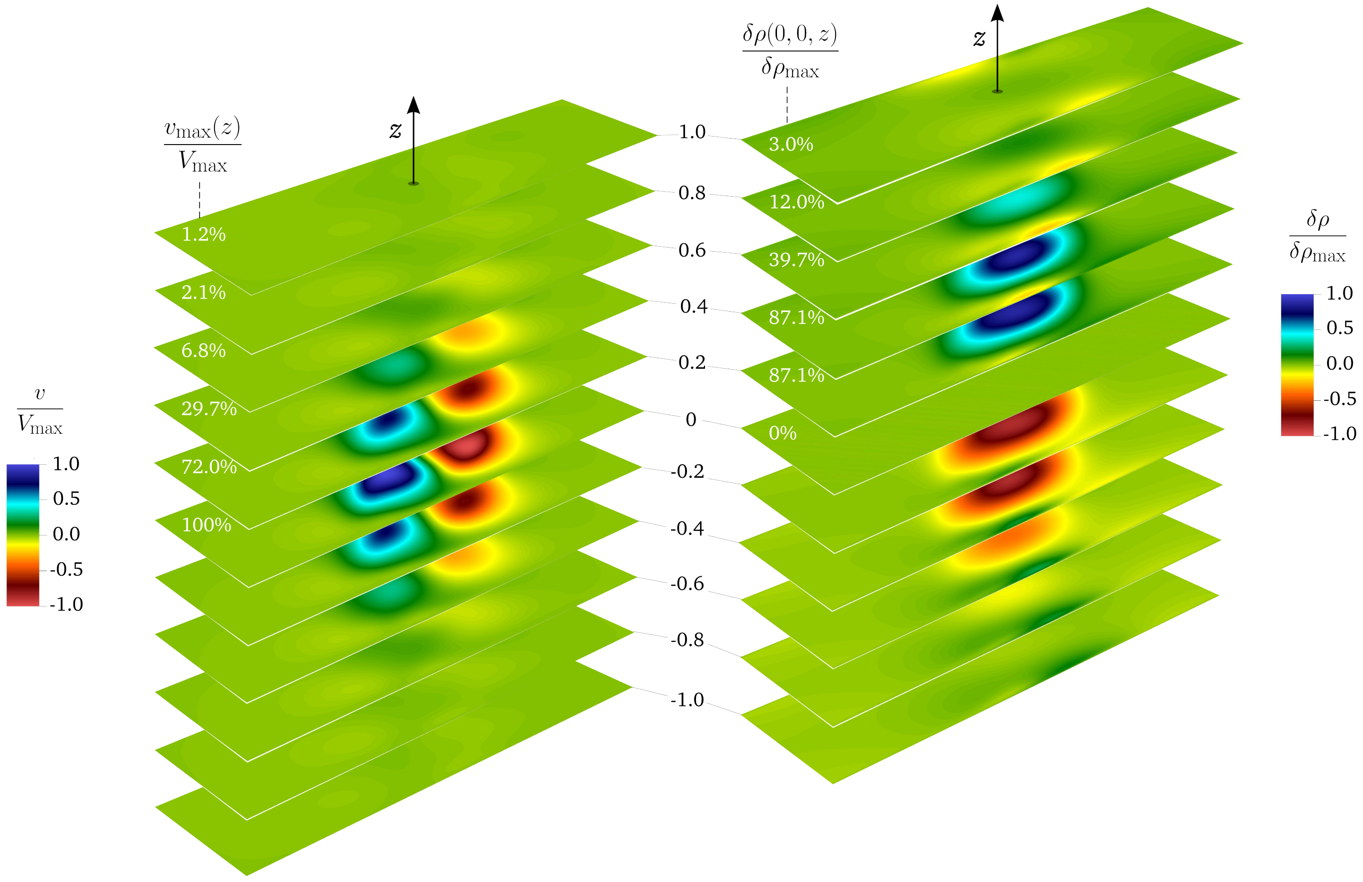


**Figure S8:** Vertical structure of the vortex for the reference simulation (Table S1) at time $t \approx 10$. The cross-stream velocity $v$ (left) and the density perturbation $\delta\rho$ (right) are represented on 11 horizontal slices for $z \in [-1, 1]$. The percentages are the ratio of the maximum velocity or density anomaly for a given slice relatively to the maximum velocity or density anomaly in the whole 3D-box.

[9] Griffiths, R. W. & Linden, P. F. The stability of vortices in a rotating, stratified fluid. *Journal of Fluid Mechanics* **105**, 283 (1981).

[10] Hedstrom, K. & Armi, L. An experimental study of homogeneous lenses in a stratified rotating fluid. *Journal of Fluid Mechanics* **191**, 535 (1988).

[11] Nguyen, H. Y., Hua, B. L., Schopp, R. & Carton, X. Slow quasigeostrophic unstable modes of a lens vortex in a continuously stratified flow. *Geophysical & Astrophysical Fluid Dynamics* **106**, 305–319 (2012).

[12] Negretti, M. E. & Billant, P. Stability of a Gaussian pancake vortex in a stratified fluid. *Journal of Fluid Mechanics* **718**, 457–480 (2013).

[13] Lazar, A. *et al.* Inertial instability of intense stratified anticyclones. Part 2. Laboratory experiments. *Journal of Fluid Mechanics* **732**, 485–509 (2013).

[14] Lazar, A., Stegner, A. & Heifetz, E. Inertial instability of intense stratified anticyclones. Part 1. Generalized stability criterion. *Journal of Fluid Mechanics* **732**, 457–484 (2013).

[15] Lahaye, N. & Zeitlin, V. Centrifugal, barotropic and baroclinic instabilities of isolated ageostrophic anticyclones in the two-layer rotating shallow water model and their nonlinear saturation. *Journal of Fluid Mechanics* **762**, 5–34 (2015).

[16] Yim, E., Billant, P. & Ménesguen, C. Stability of an isolated pancake vortex in continuously stratified-rotating fluids. *Journal of Fluid Mechanics* **801**, 508–553 (2016).

[17] Yim, E. *Stability of Columnar and Pancake Vortices in Stratified-Rotating Fluids*. Ph.D. thesis, École Polytechnique (2015).

[18] Miyazaki, T. Elliptical instability in a stably stratified rotating fluid. *Physics of Fluids A: Fluid Dynamics* **5**, 2702–2709 (1993).

[19] Chomaz, J.-M., Ortiz, S., Gallaire, F. & Billant, P. Stability of Quasi-Two-Dimensional Vortices. In Flor, J.-B. (ed.) *Fronts, Waves and Vortices in Geophysical Flows*, Lecture Notes in Physics, 35–59 (Springer Berlin Heidelberg, Berlin, Heidelberg, 2010).

[20] Guimbard, D., Le Dizès, S., Le Bars, M., Le Gal, P. & Leblanc, S. Elliptic instability of a stratified fluid in a rotating cylinder. *Journal of Fluid Mechanics* **660**, 240–257 (2010).

[21] Rogers, J. *The Giant Planet Jupiter*, vol. 6 (Cambridge University Press, 1995).

[22] Shetty, S., Asay-Davis, X. S. & Marcus, P. S. On the Interaction of Jupiter's Great Red Spot and Zonal Jet Streams. *Journal of the Atmospheric Sciences* **64**, 4432–4444 (2007).

[23] Choi, D., Banfield, D., Gierasch, P. & Showman, A. Velocity and vorticity measurements of Jupiter's Great Red Spot using automated cloud feature tracking. *Icarus* **188**, 35–46 (2007).

[24] Simon, A. A. *et al.* Historical and Contemporary Trends in the Size, Drift, and Color of Jupiter's Great Red Spot. *The Astronomical Journal* **155**, 151 (2018).

[25] Choi, D. S., Showman, A. P. & Vasavada, A. R. The evolving flow of Jupiter's White Ovals and adjacent cyclones. *Icarus* **207**, 359–372 (2010).

[26] Mitchell, J. L., Beebe, R. F., Ingersoll, A. P. & Garneau, G. W. Flow fields within Jupiter's Great Red Spot and white oval BC. *Journal of Geophysical Research: Space Physics* **86**, 8751–8757 (1981).

[27] Simon, A. A., Beebe, R. F., Gierasch, P. J., Vasavada, A. R. & Belton, M. J. S. Global Context of the Galileo-E6 Observations of Jupiter's White Ovals. *Icarus* **135**, 220–229 (1998).

[28] Asay-Davis, X. S., Marcus, P. S., Wong, M. H. & de Pater, I. Jupiter's shrinking Great Red Spot and steady Oval BA: Velocity measurements with the 'Advection Corrected Correlation Image Velocimetry' automated cloud-tracking method. *Icarus* **203**, 164–188 (2009).

[29] Limaye, S. S. Jupiter: New estimates of the mean zonal flow at the cloud level. *Icarus* **65**, 335–352 (1986).

[30] Tollefson, J. *et al.* Changes in Jupiter's Zonal Wind Profile preceding and during the Juno mission. *Icarus* **296**, 163–178 (2017).

[31] Conrath, B. J., Flasar, F. M., Pirraglia, J. A., Gierasch, P. J. & Hunt, G. E. Thermal structure and dynamics of the Jovian atmosphere 2. Visible cloud features. *Journal of Geophysical Research: Space Physics* **86**, 8769–8775 (1981).

[32] Flasar, F. M. *et al.* Thermal structure and dynamics of the Jovian atmosphere 1. The great red spot. *Journal of Geophysical Research: Space Physics* **86**, 8759–8767 (1981).

[33] Fletcher, L. N. *et al.* Thermal structure and composition of Jupiter's Great Red Spot from high-resolution thermal imaging. *Icarus* **208**, 306–328 (2010).

[34] Seiff, A. *et al.* Thermal structure of Jupiter's atmosphere near the edge of a 5-$M$m hot spot in the north equatorial belt. *Journal of Geophysical Research: Planets* **103**, 22857–22889 (1998).

[35] De Pater, I. *et al.* Persistent rings in and around Jupiter's anticyclones–Observations and theory. *Icarus* **210**, 742–762 (2010).

[36] Morales-Juberıás, R., Sánchez-Lavega, A. & Dowling, T. E. EPIC simulations of the merger of Jupiter's White Ovals BE and FA: Altitude-dependent behavior. *Icarus* **166**, 63–74 (2003).

[37] Legarreta, J. & Sánchez-Lavega, A. Vertical structure of Jupiter's troposphere from nonlinear simulations of long-lived vortices. *Icarus* **196**, 184–201 (2008).

[38] Shetty, S. & Marcus, P. S. Changes in Jupiter's Great Red Spot (1979–2006) and Oval BA (2000–2006). *Icarus* **210**, 182–201 (2010).
